# Supplementary material for: Interactions between two C60 molecules measured by scanning probe microscopies
Source: arXiv:1704.08466 source file (2017-04-27)
Supplement: Supplementary file 1 [file C60C60_Supplemental_Material.pdf]

# Supplemental Material: Interactions between two $C_{60}$ molecules measured by scanning probe microscopies

**Nadine Hauptmann[1,4], César González[2], Fabian Mohn[3], Leo Gross[3], Gerhard Meyer[3], Richard Berndt[1]**

[1]Institut für Experimentelle und Angewandte Physik,
Christian-Albrechts-Universität zu Kiel, D-24098 Kiel, Germany

[2]Departamento de Fisica, Facultad de Ciencias, 33006. Universidad Oviedo, Spain

[3]IBM Research – Zurich, CH-8803 Rüschlikon, Switzerland

[4]Institute for Molecules and Materials, Radboud University, 6500 GL Nijmegen, The Netherlands

E-mail: `n.hauptmann@science.ru.nl`

## 1. Calculated force contributions

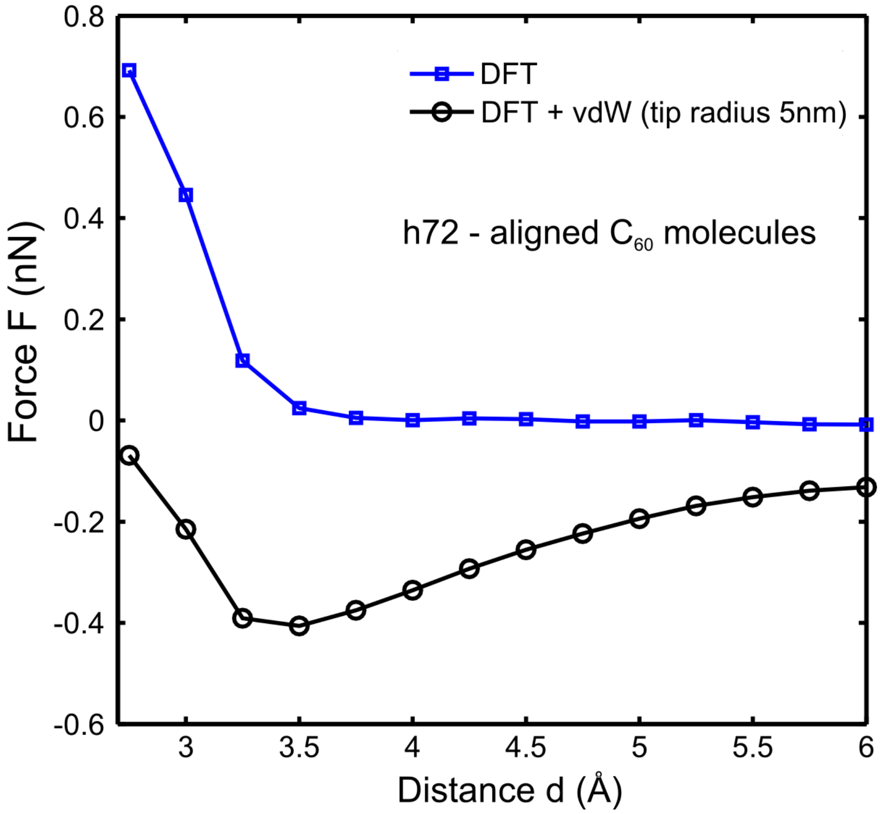


**Figure S1.** Comparison of the force without and with vdW contribution for the h72 orientation. The $C_{60}$ molecules at the tip and on the surface are aligned. The van der Waals (vdW) interaction was estimated by a semi-empirical correction based on the London expression [1]. The force contribution without the vdW interaction does not exhibit an attractive regime showing that the VdW interaction is mainly responsible for the attraction between two $C_{60}$ molecules.

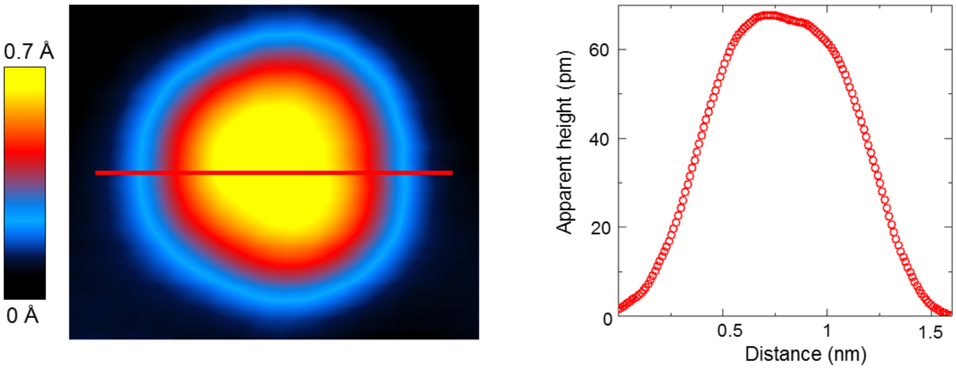


**Figure S2.** Left: STM topograph ($1.7 \times 1.4$ nm$^2$, 2 V) of a typical Cu cluster acquired with a metallic tip. Clusters were deposited by approaching the tip to the surface by several Angstroms. Right: Line profile taken along the red line in the STM image. The apparent height and lateral dimensions suggest that the cluster is comprised of a few (presumably three) atoms [2].

## References

[1] Ortmann F, Bechstedt F and Schmidt W G 2006 *Phys. Rev. B* **73** 205101

[2] Sperl A, Kröger J, Néel N, Jensen H, Berndt R, Franke A and Pehlke E 2008 *Phys. Rev. B* **77** 085422
